# Supplementary material for: Tamed Warping Network for High-Resolution Semantic Video Segmentation
Source: arXiv:2005.01344 source file (2023-07-11)
Supplement: Supplementary file 1 [file abstract.tex]

\begin{abstract}
This document provides supplemental material for \textit{\headline}.
\end{abstract}
